# Supplementary material for: RAVEN: Rethinking Adversarial Video Generation with Efficient Tri-plane Networks
Source: arXiv:2401.06035 source file (2024-08-11)
Supplement: Supplementary file 1 [file sup_mat.tex]

\clearpage
\setcounter{page}{1}
\maketitlesupplementary

\section{Real Data} Along with this PDF in our supplementary material, you will find a .zip archive that holds sample videos from our training dataset. Note that we face similar problems finding suitable data as noted in~\cite{brooks2022generating,skorokhodov2022stylegan}. The problems namely are — modern datasets of videos are either too small (only a few 100s videos (Fashion videos, FaceForensics, CelebV-HQ)), too simple ((Synthetically generated videos of NeRF objects)No object articulation, only camera motion, etc.), or too complex (very wide collection of videos of random scenes (Kinetics-600, UCF-101)). Therefore, we use clever `animation' techniques to increase data volume, as described in~\cref{subsec:datasets}. However, the methods we use are not perfect and produce artifacts depending upon the source-appearance and motion. Furthermore, we found with a manual inspection that these methods~\cite{zhao2022thin,yu2023bidirectionally}, although state-of-the-art, have the effect of generating videos with limited motion. This is then carried over to the final result of our method. Therefore, for manual judgment of generation quality, we highly recommend an inspection of the training data. In the directory named real\_samples, there are $3$ subdirectories, each containing $32$ random sample videos corresponding to each dataset.

\section{Generated data} In the directory named generated\_samples, there are $5$ subdirectories corresponding to each of the models we train. Each of these subdirectories in tern contains $3$ directories corresponding to each dataset, and each of them contains $32$ random sample videos.

\section{Extrapolation with triplane representation}
\begin{table*}[h!]
\centering
    \begin{tabular}{lcccccccccccc}
        \toprule
        & \multicolumn{4}{c}{Talking Faces all Motions} & \multicolumn{4}{c}{Fashion Videos} & \multicolumn{4}{c}{UCF 101} \\
        \cmidrule(lr){2-5} \cmidrule(lr){6-9} \cmidrule(lr){10-13}
        Method     & \multicolumn{2}{c}{3 frame interp.} & \multicolumn{2}{c}{8 frame intrp.}& \multicolumn{2}{c}{3 frame interp.} & \multicolumn{2}{c}{8 frame intrp.}& \multicolumn{2}{c}{3 frame interp.} & \multicolumn{2}{c}{8 frame intrp.} \\ 
        \cmidrule(lr){2-3}\cmidrule(lr){4-5}\cmidrule(lr){6-7}\cmidrule(lr){8-9}\cmidrule(lr){10-11}\cmidrule(lr){12-13}
         & SSIM & PSNR & SSIM & PSNR & SSIM & PSNR & SSIM & PSNR & SSIM & PSNR & SSIM & PSNR \\
        \midrule
        Pos. emb & 0.17 &15.26 &0.17 &15.19 &0.70 &17.41 &0.70 &17.59 &0.17 &14.29 &0.21 &14.39  \\
        voxels & 0.73 &25.71 &0.71 &24.77 &0.86 &24.87 &0.85 &23.95 &0.46 &19.54 &0.46 &19.57  \\
        triplane  & 0.83 &28.49 &0.82 &27.61 &0.91 &27.65 &\textbf{0.90} &26.40 &0.50 &19.87 &0.50 &19.88  \\
        triplane+flow & \textbf{0.86} &\textbf{29.76} &\textbf{0.84} &\textbf{28.32} &\textbf{0.92} &\textbf{28.25} &\textbf{0.90} &\textbf{26.65} &\textbf{0.51} &\textbf{20.25} &\textbf{0.52} &\textbf{20.11}  \\
        \bottomrule
    \end{tabular}
    \caption{\textbf{Tri-plane video representation for extrapolation:} We compare the effectiveness of the tri-plane representation for Video data by computing SSIM and PSNR value of extrapolated frames. Note that for all metric, higher is better. The reported numbers here are average PSNR over $20$ random videos taken from each of our data sets}
    \label{table:quantitative_comaprison_extrapolation}
\end{table*}
